# Supplementary material for: PAS : Prelim Attention Score for Detecting Object Hallucinations in Large Vision--Language Models
Source: arXiv:2511.11502 source file (2025-11-14)
Supplement: Supplementary file 1 [file algo.tex]

% In your preamble (if not already included):
% \usepackage[ruled,vlined]{algorithm2e}

%---------------------- Algorithm 1: Offline Calibration (A → B) ----------------------
\begin{algorithm}[t]
\small
\DontPrintSemicolon
\SetAlgoNoLine
\SetKwInOut{Input}{Input}
\SetKwInOut{Output}{Output}
\caption{\textbf{Offline Calibration for PAL (A $\rightarrow$ B)}}
\label{alg:calibration}
\Input{
LVLM $\Phi$; early layer $l^\star$; object vocabulary $\mathcal{V}_{\text{obj}}$;\\
Calibration set $\mathcal{D}=\{(I,t)\}$; optional image pools $\{\mathcal{I}(c)\}$ per class $c$;\\
Decoding params (e.g., greedy, $\texttt{max\_new\_tokens}$).
}
\Output{
Monotonic calibration $g$ (optional), threshold $\tau$ for deployment.
}
\BlankLine
$\mathcal{S}\leftarrow \varnothing$ \tcp{store tuples for calibration}
\ForEach{$(I,t)\in \mathcal{D}$}{
  \tcp{Single forward pass to read native attention tensors}
  $(\mathbf{y}, \{\mathbf{A}^{(l,h)}\}_{l,h}) \leftarrow \Phi\text{-}\textsc{Forward}(I,t)$\;
  $\mathcal{J}_{\text{obj}} \leftarrow \textsc{ExtractObjectMentions}(\mathbf{y}, \mathcal{V}_{\text{obj}})$\;
  \ForEach{$k \in \mathcal{J}_{\text{obj}}$}{
    \tcp{B-path: fast prelim-attention score at early layer $l^\star$}
    $s_{\text{prel}}(y_k) \leftarrow \frac{1}{H}\sum_{h=1}^H\sum_{j=m+1}^{k} \mathbf{A}^{(l^\star,h)}(k,j)$\;
    \tcp{A-path: slow, theory-inspired contrast (optional)}
    $c \leftarrow \textsc{ClassOf}(y_k)$\;
    $f_A(y_k) \leftarrow \textsc{TheoryContrast}\big(y_k, t, \mathcal{I}(c)\big)$\;
    \tcp{Label via benchmark annotation (e.g., CHAIR/POPE protocol)}
    $\ell_k \leftarrow \textsc{IsHallucinated}(y_k, I)$\;
    $\mathcal{S} \leftarrow \mathcal{S}\cup \{(s_{\text{prel}}(y_k), f_A(y_k), \ell_k)\}$\;
  }
}
\tcp{Fit a monotonic map $g$ or a logistic model from $s_{\text{prel}}$ to $f_A$ or $\Pr(\text{halluc})$}
$g \leftarrow \textsc{IsotonicOrLogisticFit}(\{(s_{\text{prel}}, f_A)\in \mathcal{S}\})$ \;
\tcp{Pick operating threshold $\tau$ (e.g., maximize dev F1 or Youden’s $J$)}
$\tau \leftarrow \arg\max_{\tau'} \ \textsc{F1}\big(\mathbf{1}[g(s_{\text{prel}})\ge \tau'], \ell \big)$ using $\mathcal{S}$\;
\Return{$g,\ \tau$}\;
\end{algorithm}

%\vspace{4pt}
%\noindent\textbf{Helpers (sketch).}
%\begin{itemize}\itemsep3pt
%\item $\textsc{ExtractObjectMentions}$: string-match surface forms from $\mathcal{V}_{\text{obj}}$ over detokenized $\mathbf{y}$; collapse BPE spans to the last subtoken position $k$ representing the object mention.
%\item $\textsc{TheoryContrast}$: compute $f_A(y_k)=\Delta(\Pr(y_k\mid \mathbf{y}_{\le k},t),\Pr(y_k\mid \mathbf{x}))$ via extra passes / perturbations / Monte Carlo over $\mathcal{I}(c)$ (slow, offline).
%\end{itemize}

%---------------------- Algorithm 2: Runtime Detection (PAL, fast) ----------------------
\begin{algorithm}[t]
\small
\DontPrintSemicolon
\SetAlgoNoLine
\SetKwInOut{Input}{Input}
\SetKwInOut{Output}{Output}
\caption{\textbf{Runtime PAL (single pass)}}
\label{alg:runtime}
\Input{
LVLM $\Phi$; early layer $l^\star$; object vocabulary $\mathcal{V}_{\text{obj}}$;\\
Calibration $(g,\tau)$ from Alg.~\ref{alg:calibration}; image $I$, prompt $t$.
}
\Output{
Token-level scores and flags $\{(k, s_{\text{prel}}(y_k), \hat{\ell}_k)\}$; optional caption-level flag.
}
\BlankLine
$(\mathbf{y}, \{\mathbf{A}^{(l,h)}\}_{l,h}) \leftarrow \Phi\text{-}\textsc{Forward}(I,t)$ \tcp*{one pass}
$\mathcal{J}_{\text{obj}} \leftarrow \textsc{ExtractObjectMentions}(\mathbf{y}, \mathcal{V}_{\text{obj}})$\;
\ForEach{$k \in \mathcal{J}_{\text{obj}}$}{
  $s_{\text{prel}}(y_k) \leftarrow \frac{1}{H}\sum_{h=1}^H\sum_{j=m+1}^{k} \mathbf{A}^{(l^\star,h)}(k,j)$\;
  $\tilde{s}_k \leftarrow g(s_{\text{prel}}(y_k))$ \tcp*{optional calibrated score}
  $\hat{\ell}_k \leftarrow \mathbf{1}[\tilde{s}_k \ge \tau]$ \tcp*{flag hallucinated token}
}
\tcp{Optional caption-level aggregation (e.g., flag if any token flagged)}
$\hat{\ell}_{\text{cap}} \leftarrow \mathbf{1}\big[\exists k\in \mathcal{J}_{\text{obj}}: \hat{\ell}_k=1\big]$\;
\Return{$\{(k, s_{\text{prel}}(y_k), \hat{\ell}_k)\},\ \hat{\ell}_{\text{cap}}$}\;
\end{algorithm}

%---------------------- Notes ----------------------
% Complexity notes (optional to include near the algorithms):
% - No extra forward passes at runtime; we read attention already computed by \Phi.
% - Per object token y_k, computing s_prel is O(H \cdot (k-m)) summation over heads and prelim positions.
% - Memory overhead is negligible beyond storing the layer-l^\star attention for one pass.
